# Supplementary material for: Combining Pessimism with Optimism for Robust and Efficient Model-Based Deep Reinforcement Learning
Source: arXiv:2103.10369 source file (2021-03-18)
Supplement: Supplementary file 1 [file drrl.tex]

%!TEX root = ./../main.tex
% \section{Attempt to Formalize Distributionally Robust Objective}
% Comment: In case we agree this is useful, we can incorroporate it in the main text/appendix.

% We consider the following dynamics model:
% \begin{equation}
% 	\x_{\hi+1} = f(\x_\hi, \u_\hi, c) + \noise_\hi,
% \end{equation}
% where $c$ is assumed to be sampled i.i.d. from some unknown $Q^*$. To make things simpler we can assume $c$ is the same for every $n$. Here, $c$ represents a random context parameter, e.g., weather condition that can impact transition dynamics -- when breaking, an autonomous vehicle might end up in a different state depending on whether it is raining or not.

% We consider the following learning protocol. At every episode $\ti$:
% 	\begin{enumerate}
%         \item The agent selects $\pi_\ti$;
%         \item The environment draws $c_\ti \sim Q^*$ independently;
%         \item The policy $\pi_\ti$ is deployed on the true system $f(\cdot,\cdot, c_\ti)$;
%         \item Agent receives a realization of the trajectory $\tau_{f, \pi_\ti, c_\ti}$.
%     \end{enumerate}

% We define the performance as follows:
% \begin{align}
%         J(f, \pi, Q^*) &\coloneqq \E[\tau_{\tilde{f}, \pi}, c\sim Q^*]{\sum_{\hi=0}^{\Hi} r(\x_\hi, \u_\hi, c) \, \bigg| \, \x_0}. 
% \end{align}

% The stochastic optimization, i.e., contextual objective (also not explicitly considered before in the model-based/kernelized setting, as far as I know) is:
% \begin{equation}
%         \pi^* = \max_{\pi \in \Pi} J(f, \pi, Q^*).
%         \label{eq:stochastic_policy}  
% \end{equation}
% We can tackle this non-robust contextual problem as well.

% Next, the distributionally robust objective, can be formalized as follows. Define some $\mathcal{U}_t(\hat{Q}_t, \epsilon_t)$ uncertainty set at time $t$, i.e., all the distributions that are at most $\epsilon_t$--far from $\hat{Q}_t$.  As benchmark, consider the optimal robust policy with respect to this set: 
% \begin{equation}
%     \pi^*_t = \max_{\pi \in \Pi} \min_{Q \in \mathcal{U}_t(Q_t,\epsilon_t)} J(f, \pi, Q).  
% \end{equation}
% Basically, this is the optimal robust policy with respect to knowledge that we have of the true distribution $Q^*$ at time $t$. When selecting our policy $\pi_t$, we assume the knowledge of $\mathcal{U}_t$. As $t$ grows large, we have $\hat{Q}_t$ (empirical distribution) converges to the true distribution $Q^*$, and consequently, we can consider a shrinking sequence of $\lbrace \epsilon_i \rbrace_{i=1}^T$. We also observe that as $t \to \infty$, we have $\pi^*_t$ approaches $\pi^*$ defined in \eqref{eq:stochastic_policy}.

% By considering robust cumulative regret, our goal is select a policy that is robust at every time step, where the robustness is with respect to our current uncertainty about the unknown $Q^*$:
% \begin{equation}
% 	\sum_{t=1}^T \Big(\min_{Q \in \mathcal{U}_t(Q_t,\epsilon_t)} J(f, \pi^*_t, Q) - \min_{Q \in \mathcal{U}_t(Q_t,\epsilon_t)} J(f, \pi_t, Q) \Big).
% \end{equation}  
